# Supplementary material for: Balance functions of charged hadron pairs $(\pi,K,p)\otimes (\pi,K,p)$ in Pb--Pb collisions at $\sqrt{s_{_{\rm NN}}} =$2.76 TeV
Source: arXiv:1911.02234 source file (2019-11-06)
Supplement: Supplementary file 1 [file appendix_a.tex]

\chapter{Appendix A name}\label{app:appAlabel}

%\titleformat
%{\chapter} % command
%[hang] % shape
%% Add \singlespacing here if it's a problem
%{\normalfont\normalsize\bfseries\center} % format
%{} % label
%{0pt} % sep
%{\MakeUppercase} % before code

% Sample figure, table, and equation:

%\begin{figure}
%\begin{center}
%\includegraphics*[width=16.5cm]{plots/somefile.eps}
%\end{center}
%\caption{A caption}
%\label{fig:figurereference1}
%\end{figure}

%\begin{table}[htb]
%\caption{Table caption.
%\label{tab:tablereference1}}
%\begin{center}
%\begin{tabular}{cc}
%\hline
%Symbol & Name \\
%\hline
%{\it u} & Up \\
%{\it d} & Down \\
%\hline
%{\it c} & Charm \\
%{\it s} & Strange \\
%\hline
%{\it t} & Top \\
%{\it b} & Bottom \\
%\hline
%\end{tabular}
%\end{center}
%\end{table}

%\begin{equation}
%n \to p + e^- + \bar{\nu}_e
%\label{eq:equationreference1}
%\end{equation}
