# Supplementary material for: Balance functions of charged hadron pairs $(\pi,K,p)\otimes (\pi,K,p)$ in Pb--Pb collisions at $\sqrt{s_{_{\rm NN}}} =$2.76 TeV
Source: arXiv:1911.02234 source file (2019-11-06)
Supplement: Supplementary file 2 [file appendix_header.tex]

%\renewcommand\chaptername{APPENDIX}                      % hereafter, chapters are called "Appendix"
%\renewcommand\thechapter{\Alph{chapter}}                % chapter number in alph letters
%\renewcommand\thesection{\Alph{chapter}.\Roman{section}} % make sections "A.I"
%\setcounter{chapter}{0}                                  % start numbering chapters from 1 on again
\appendix
